# Supplementary material for: The silver route to cuprate analogs
Source: arXiv:1804.00329 ancillary file (2018-04-01)
Supplement: Supplementary file 1 [file SI.pdf]

# Supplementary Materials for The silver route to cuprate analogs

Jakub Gawraczyński,<sup>1,2</sup> Dominik Kurzydłowski,<sup>1,3</sup> Wojciech Gadomski,<sup>2</sup>  
Zoran Mazej,<sup>4</sup> Giampiero Ruani,<sup>5</sup> Ilaria Bergenti,<sup>5</sup> Tomasz Jaroń,<sup>1</sup>  
Andrew Ozarowski,<sup>6</sup> Stephen Hill,<sup>6,7</sup> Piotr J. Leszczyński,<sup>1</sup> Kamil Tokár,<sup>8</sup>  
Mariana Derzsi,<sup>1</sup> Paolo Barone,<sup>9</sup> Krzysztof Wohlfeld,<sup>10</sup>  
José Lorenzana,<sup>11\*</sup> Wojciech Grochala<sup>1\*</sup>

<sup>1</sup> Center of New Technologies, University of Warsaw,  
Żwirki i Wigury 93, 02089 Warsaw Poland

<sup>2</sup> Faculty of Chemistry, University of Warsaw, Pasteur 1, 02093 Warsaw Poland

<sup>3</sup> Faculty of Mathematics and Natural Sciences, Cardinal Stefan Wyszyński  
University in Warsaw, Wóycickiego 1/3, 01938 Warsaw Poland

<sup>4</sup> Department of Inorganic Chemistry and Technology,  
Jožef Stefan Institute, Jamova 39, SI-1000 Ljubljana, Slovenia

<sup>5</sup> Institute of Nanostructured Materials, ISMN-CNR, via Gobetti 101, 40129 Bologna, Italy

<sup>6</sup> National High Magnetic Field Laboratory, Florida State University,  
1800 E. Paul Dirac Drive, Tallahassee, Florida 32310, USA

<sup>7</sup> Department of Physics, Florida State University,  
Tallahassee, Florida 32306, USA

<sup>8</sup> Institute of Physics, Slovak Academy of Sciences, Dúbravská cesta 9, Bratislava, Slovakia

<sup>9</sup> Superconducting and other Innovative Materials and Devices Institute,  
SPIN-CNR, via Vetoio, 67100 L'Aquila, Italy

<sup>10</sup> Faculty of Physics, University of Warsaw, Pasteur 5, 02093 Warsaw Poland

<sup>11</sup> Institute for Complex Systems, ISC-CNR, Dipartimento di Fisica,  
Università di Roma "La Sapienza", Piazzale Aldo Moro 5, 00185 Roma, Italy

\*To whom correspondence should be addressed;

E-mail: jose.lorenzana@cnr.it, w.grochala@cent.uw.edu.pl.

# Materials and Methods

## Structure

Visualization of the structure has been performed with the use of the VESTA software (31). Crystal structure of  $\text{AgF}_2$  has been described in detail before based on powder neutron data (32–34). At ambient conditions  $\text{AgF}_2$  crystallizes in a distorted rutile-type structure of orthorhombic symmetry. This structure contains puckered  $\text{AgF}_2$  sheets containing corner sharing  $\text{AgF}_4$  plaquettes. The octahedral coordination of  $\text{Ag}^{2+}$  is completed by two fluorine atoms from neighbouring sheets. This structure can thus be described as built of puckered 2D sheets. Figure S1 compares the structure of  $\text{AgF}_2$  and a typical cuprate.

## DFT computations

Unpolarized DFT calculations have been performed using the projector-augmented waves (PAW) method as implemented in VASP (35) within the generalized-gradient approximation of Perdew, Burke, and Ernzerhof (36) (PBE) and the crystal structure of Ref. 37. The band structure was obtained for the experimental lattice (37) using a Monkhorst-Pack mesh of  $26 \times 26 \times 26$   $k$ -points and a 500 eV plane-wave cutoff. A smaller mesh of  $8 \times 8 \times 8$   $k$ -points has been used for the projection onto maximally-localized Wannier functions. Polarized computations were done with the HSE06 functional (38) which is a hybrid functional mixing PBE with 25% of Hartree-Fock (HF) exchange energy.

For the phonon assignments, dynamical matrix inter-atomic force constants and polarizabilities (macroscopic dielectric tensors) for computing IR and Raman intensities were obtained from the density-functional perturbation theory (DFPT) scheme with  $(6 \times 6 \times 7)$   $k$ -point mesh (including 64 irreducible points) and cutoff = 520 eV, using PBEsol functional in combination with Hubbard U for  $\text{Ag}^{2+}$  ions with one unpaired electron (electronic configuration  $3d^9$ ) within DFT+U scheme as implemented in the VASP package (35). The Hubbard  $U_{\text{Ag}}$  was set to 5 eV and  $J_H$  to 1 eV.

The  $\Gamma$ -point vibrational frequencies were calculated by diagonalizing the dynamical matrix for the fully converged structural  $\text{AgF}_2$  model. IR intensity of vibrational eigenmodes has been expressed within dipole approximation in terms of atoms born effective charges and corresponding phonon eigenvectors using the formula for modal oscillator strengths (39, 40) as implemented in Ref. 41. Intensity of each Raman mode was calculated from cross-section formula and spatially averaged from the polarization tensor element derivatives accessible directly from DFPT as implemented in Ref. 42. The electronic and ionic convergence was restricted to  $10^{-8}$  eV and  $10^{-7}$  eV, respectively. The atomic forces were converged to maximal value of 0.02 meV/Å.

## Five-band Hubbard model for AgF<sub>2</sub>.

As for cuprates (43), one can consider a simplified model of the electronic structure of AgF<sub>2</sub> in which the more relevant  $d$  and  $p$  orbitals are taken into account. Since accurate values of electronic parameters are not available for  $d^9$  Ag compounds, our aim here is to provide estimates of the more important parameters that determine the magnetic interaction in AgF<sub>2</sub>. In addition, we discuss the similarities and difference of the parameters with cuprates and show that a large value of the magnetic interaction in AgF<sub>2</sub> is compatible with the parameter estimates.

A natural choice for a minimal model, is to consider one  $d_{x^2-y^2}$  orbital per Ag. For the F's, due to the strongest buckling respect to cuprates, one should consider one extra  $p$ -orbital per fluorine atom which mixes significantly with the  $d$ -orbital. Figure S2 shows schematically a silver-fluorine-silver (L-F-R) bond and defines the more relevant orbitals. Here, L and R are left and right silver ions and F refers to the bridging fluoride. We call  $\eta$  the L-F-R angle. Orbitals are defined in the caption. In the room temperature structure (37)  $\eta = 129.9^\circ$ .

By symmetry, the  $p_\perp$  orbital taken in the direction of the red arrow in Figure S2 has negligible mixing with the  $d_{L/R}$  orbitals. Therefore, we restrict to two  $p$  orbitals for the central F, namely  $p_\parallel$  parallel to the L-R line (green arrow) and  $p_z$  in the plane that contains the L-F-R triangle and perpendicular to the bond (blue arrow).

For the lattice, since there are two fluorine atoms per f.u. one should consider a five-band Hubbard model rather than the usual (43) three-band Hubbard model of cuprates. The model reads  $H = H_1 + H_2$  with,

$$H_1 = \sum_{i,\sigma} e_i c_{i\sigma}^\dagger c_{i\sigma} + \sum_{i \neq j, \sigma} t_{ij} c_{i\sigma}^\dagger c_{j\sigma}, \quad (\text{S1})$$

$$H_2 = \sum_i U_i c_{i\downarrow}^\dagger c_{i\downarrow} c_{i\uparrow}^\dagger c_{i\uparrow} + \sum_{\langle i \neq j \rangle, \sigma, \sigma'} U_{ij} c_{j\sigma'}^\dagger c_{j\sigma'} c_{i\sigma}^\dagger c_{i\sigma} + \sum_{\langle i \neq j \rangle, \sigma, \sigma'} K_{ij} c_{i\sigma}^\dagger c_{i\sigma'} c_{j\sigma'}^\dagger c_{j\sigma}, \quad (\text{S2})$$

where the operator  $c_{i\sigma}^\dagger$  creates a *hole* of spin  $\sigma$  and the index  $i$  runs through the Ag  $d_{x^2-y^2}$  and the F  $p_{\parallel,z}$  orbitals defined in Supplementary Fig. S2.  $e_i$  and  $t_{ij}$  are single particle and hopping matrix elements respectively. Holes repel each other with strength  $U_i$  on orbital  $i$  and strength  $U_{ij}$  between different orbitals  $i$  and  $j$ .  $K_{ij}$  is the direct exchange interaction between different orbitals (usually ferromagnetic, i.e.  $K_{ij} < 0$ ).

## Estimate of hopping matrix elements

We discuss the more relevant hopping matrix elements for the nearest-neighbor magnetic interaction. Other matrix elements and further details will be presented elsewhere. We define  $t_{pd}$  as the hopping matrix element of an hypothetical straight L-F-R bond ( $\eta = 180^\circ$ ) keeping the Ag-F distances constant. In this case only the  $p_\parallel$  orbital mixes significantly and the hopping matrix element is  $t_{pd} \equiv (\sqrt{3}/2)(pd\sigma)$  where  $(pd\sigma)$  is the usual Slater-Koster (44) parameter. We find that  $(pd\pi)$  matrix elements do not play an important role therefore, as customary for cuprates, we neglect them in the present computation.

Referring to Supplementary Fig. S2, matrix elements are defined by the following equations,

$$\begin{aligned} H_1|d_L\rangle &= -t_{\parallel d}|p_{\parallel}\rangle + t_{zd}|p_z\rangle, \\ H_1|d_R\rangle &= t_{\parallel d}|p_{\parallel}\rangle + t_{zd}|p_z\rangle, \end{aligned} \quad (\text{S3})$$

where we introduced,

$$t_{\parallel d} \equiv t_{pd} \sin(\eta/2), \quad t_{zd} \equiv t_{pd} \cos(\eta/2). \quad (\text{S4})$$

We can obtain a first estimate of the straight-bond parameter  $t_{pd}$  from band structure computations in related compounds. Refs. 45, 46 report  $t_{pd}$  for hypothetical solids with various F-Ag distances. We have estimated  $t_{pd}$  in  $\text{AgF}_2$  using the scaling of Ref. 47 to extrapolate to the equilibrium bond distances in  $\text{AgF}_2$  (Supplementary Fig. S4) and obtained  $t_{pds} = 1.39$  eV and  $t_{pdl} = 1.37$  eV where  $s/l$  refer to the nonequivalent short (2.067 Å) and long (2.074 Å) bonds present in the structure. Using Eq. (S4), we obtain the  $pd$ -hopping matrix elements labeled “Slater-Koster” in Supplementary Table S1.

A more direct determination can be obtained by performing an unpolarized DFT computation of  $\text{AgF}_2$  followed by a parametrization of the bands in terms of Wannier orbitals which can be done using the maximally-localized projection scheme as implemented in the Wannier90 code (48). Supplementary Fig. S3 shows in red the DFT band structure in the region of the  $pd$ -bands. The blue lines are the bands obtained with the Wannier90 code with one  $d$ -like Wannier orbital centered on each Ag and two  $p$ -like Wannier orbitals centered on each F (5-band model) adopting the same local reference frame as defined in Supplementary Fig. S2. Parameters are optimized to represent as best as possible the bands that cross the Fermi level inside a “frozen” energy window (shown in Supplementary Fig. S3). Indeed, we see that this goal is well fulfilled. Other bands are not expected to be reproduced since they are dominated by orbitals not in the five-band model. In particular, as can be seen from the left panel, the bands immediately below the frozen window and above -3 eV have dominant  $p_{\perp}$  character and  $d$  character different from  $x^2 - y^2$ . Below that region significant weight in the orbitals of the five-band model appears again. This region, being far from the Fermi level is not constrained to be reproduced in detail but general features, as the overall bandwidth, is well reproduced by the Wannier parametrization, which is enough for our purpose.

We checked that the optimized orbitals obtained with Wannier90 correspond closely to the  $d_{x^2-y^2}$  and the  $p_{z,\parallel}$  orbitals defined above which confirms this simple picture. Furthermore, the values of the hopping parameters (Supplementary Table S1) corresponds fairly well (except for  $t_{dzt}$ ) with the values estimated using a single Slater-Koster parameter and structural information. If we perform the Wannier90 optimization with *all*  $d$ - and  $p$ -orbitals, one obtains a perfect fit of the DFT band structure in the whole energy window of Supplementary Fig. S3 (not shown). The resulting hoppings (last row in Supplementary Table S1) match almost perfectly the values obtained with the Slater-Koster parametrization. This indicates that the slightly different parameters of the five orbital Wannier computation, take into account indirect

hopping processes though the neglected orbitals and therefore such values are the recommended ones in a five-band model.

As with the analysis of Fig. S4 the parameter  $t_{pd}$  obtained from Wannier90 is very close to the value accepted for cuprates (49) ( $t_{pd} \sim 1.3 - 1.6$  eV) although, as will be discussed below, because of buckling the resulting magnetic interaction is smaller. Regarding in plane fluorine-fluorine hoppings we find that they are on the range  $t_{pp} \sim 0.13 - 0.3$  eV which is roughly a factor of two smaller than accepted values for oxygen-oxygen hoppings in cuprates ( $t_{pp} \sim 0.65$ ). This is expected as distances are generally larger than in cuprates and the F's orbitals are more localized than those of O's. Another important difference is that for AgF<sub>2</sub> small but non-negligibly fluorine-fluorine hoppings connect different planes in specific directions. This will result in longer-range magnetic interaction as will be clear from the polarized DFT computations.

## Estimate of the on-site repulsion and the charge transfer energy

Here we provide details of the estimate of the strength of the Coulomb interaction on the Ag 4d orbitals using the empirical information available and polarized DFT computations. In general 4d orbitals are more extended than 3d. Therefore, one would expect that the on-site Coulomb interaction in the present compound is smaller than in cuprates. As mentioned in the main text and elaborated here, poorer screening tends to compensate that.

As mention in the main text, in solids the Hubbard interaction  $U = U^0 - R$  is strongly screened respect to the free ion value,  $U^0$ , due to the relaxation of the environment. As it is well known  $R$  can be quite large, for example for the  $d$  shell of Cu,  $U_d^0 = 18.6$  eV for free ions and gets reduced to  $9 \sim 10$  eV in oxides (50–53).

A rough estimate of  $R$  can be obtained assuming that the relaxation is dominated by the polarization of the neighbors (50, 53) due to the electric field  $\pm e/d_i^2$  of added/removed electrons. Here  $d_i$  is the distance to the neighbor. This yields,

$$R = 2 \sum_i P_i, \quad (\text{S5})$$

with  $P_i = \alpha e^2 / (2d_i^4)$ . The sum runs over neighbors assumed to have polarizability  $\alpha$ . For oxygen (54)  $\alpha$  varies in the range  $\alpha_O = 0.5 \sim 3.2$  Å<sup>3</sup>. In the case of La<sub>2</sub>CuO<sub>4</sub>,  $\alpha_O \sim 1.9$  Å<sup>3</sup> is needed to obtain  $R \sim 10$  eV. Polarizabilities have units of volume and tend to scale with ionic volumes. Indeed,  $F^-$  has a smaller polarizability (54) due to the more compact orbitals,  $\alpha_F = 0.64$  Å<sup>3</sup>, and the  $d_i$  distances are smaller so Eq. (S5) yields  $R \sim 2.4$  eV for the screening of  $U_d$  in AgF<sub>2</sub>. Thus, we see that the expectation of smaller values of  $U_d$  in the 4d shell respect to the 3d shell can be compensated by poorer screening. These estimates, however, are too crude to obtain practical values of  $U_d$  in the solid and are presented only to show that expectations based on the extension of the orbitals may be too crude too.

Unfortunately, direct probes of  $U_d$  in AgF<sub>2</sub> are not available. As mentioned in the main text, estimates of solid state values can be obtained by examining experiments on closed  $d$  shell systems where Auger spectroscopy gives a direct measurement of  $U_d$  according to Cini-Sawatzky

theory (55, 56). First estimates were obtained by Powell analyzing the Auger spectra of the noble metals. We can check the relevance of this measurements for our propose comparing the case of pure Cu metal and Cu in oxides. For elementary Cu, Powell concluded that  $U_d = 7.7$  eV, similar to the value obtained by Sawatzky and collaborators (57) and somehow below to the value accepted in parent high- $T_c$  cuprates,  $U_d \sim 8 \sim 10$  eV (49, 51). The strongest screening in the metal respect to the oxide can be attributed to screening by the open  $4s$  shell.

Since Ag atom is larger than Cu atom, for elementary noble metals we expect larger polarizability and a smaller bare Coulomb integral in the former respect to the latter. Consistently  $U_d = 5.1$  eV is found in elementary Ag (58, 59), smaller than Cu but still quite large. This value should be taken as a lower bound to the value for a compound like  $\text{AgF}_2$  because of the additional screening of  $5s$  electrons.

A more realistic value of  $U_d$  for its use in  $\text{AgF}_2$  can be obtained from the analysis of Auger spectra in  $\text{Ag}_2\text{O}$  where Ag is in the  $d^{10}$  configuration. For comparison in the case of  $\text{Cu}_2\text{O}$  (also  $d^{10}$ )  $U_d = 9.2$  eV was obtained by Tjeng, Sawatzky and collaborators (52). This is close to standard value used in superconducting cuprates although in the latter case screening is expected to be larger due to the larger number of nearest neighbor O's. In the case of  $\text{Ag}_2\text{O}$ , they obtained  $U_d = 5.8$  eV which could be explained with a screening  $R = 9$  eV. This is underestimated with Eq. (S5) and  $\alpha_O = 3.2 \text{ \AA}^3$  which yields  $R = 5.2$  eV.

For  $\text{AgF}_2$ , Eq. (S5) yields  $R = 2.4$  eV. If taken literally this would imply  $U_d = 12.4$  eV, but given the above underestimation of the screening in  $\text{Ag}_2\text{O}$  we suspect that this value of  $U_d$  is too large. The physical value should be smaller than this but larger than the one found in the metal i.e.  $5.1 \text{ eV} < U_d < 12.4 \text{ eV}$ . This indicates that a value similar to the one in cuprates is quite reasonable.

An alternative estimate can be obtained from the distance between Hubbard bands in hybrid DFT and indicated with red arrows in Fig. 2. This yields  $U_d = 10.7$  eV ( $\text{La}_2\text{CuO}_4$ ) and  $U_d = 9.4$  eV ( $\text{AgF}_2$ ). For concreteness in the computations of magnetic interactions below we use the latter value. Clearly more accurate theoretical and experimental determinations are called for.

Another important parameter is the charge transfer energy  $\Delta$  which can be defined as the energy cost to transfer a hole from the  $d$  shell of the transition metal to the  $p$  shell of the ligand in the absence of hybridization, ( $d^9 + p^6 \rightarrow d^{10} + p^5$ ). We notice that the insulating gap in the hybrid DFT computation for  $\text{La}_2\text{CuO}_4$  (Fig. 2) is very close to the value of the charge transfer parameter ( $\Delta \equiv e_d - e_p$ ) estimated from constrained DFT (49) computations  $\Delta = 3.5$  eV. Thus, we use the gap in the  $\text{AgF}_2$  computation as a proxy to estimate  $\Delta = 2.7$  eV. For simplicity we neglect the crystal field splitting between the  $p$  orbitals.

Finally, given the more compact  $p$  orbitals in fluorine the bare Coulomb interaction should be larger than for oxygen but we expect this to be partially compensated by a larger screening due to a polarizability of silver larger than copper so we take  $U_p = 4$  eV, close to typical values in cuprates.

## Magnetic interactions

Our aim here is to describe the magnetic excitations of the system with a Heisenberg model,

$$H = \frac{1}{2} \sum_{ij} J_{ij} \mathbf{S}_i \cdot \mathbf{S}_j, \quad (\text{S6})$$

where the sums run over all Ag sites and  $\mathbf{S}_i$  is a spin 1/2 operator. The similarity of the parameters estimated above for  $\text{AgF}_2$  with the ones for cuprates suggest that the nearest-neighbor antiferromagnetic interaction  $J$ , should be large in the present compound. We first use perturbation theory to estimate the order of magnitude and discuss the effect of buckling for the nearest-neighbor exchange interaction. Then we present a DFT computation to examine longer range interactions and estimate the degree of anisotropy.

### Perturbative computation.

We consider again the L-F-R of Supplementary Fig. S2. The antiferromagnetic interaction among nearest-neighbor spin-1/2 Ag sites is the result of two opposite mechanisms: Anderson's superexchange (60) and direct exchange. An important point is that due to buckling the  $p_z$  orbital of Supplementary Fig. S2 cannot be neglected.

A first estimate of the nearest-neighbor interaction can be done using perturbation theory. Direct exchange appears at second order in the hopping while superexchange appears at fourth order. One obtains,  $J = J^{(2)} + J^{(4)}$ , with,

$$J^{(2)} = 2t_{\parallel d}^2 \left( \frac{1}{\Delta - K_{\parallel d}} - \frac{1}{\Delta + K_{\parallel d}} \right), \quad (\text{S7})$$

$$J^{(4)} = \frac{(t_{\parallel d}^2 - t_{zd}^2)^2}{\Delta^2} \left( \frac{4}{U_d} + \frac{8}{2\Delta + U_p} \right). \quad (\text{S8})$$

Here, given the uncertainties in parameters, we made various simplifying assumptions. We neglected the small difference in hopping matrix elements due to short and long Ag-F bonds reported in Supplementary Table S1. Similarly to the case (61) of  $\text{CuGeO}_3$ , both the Hund's rule exchange among the  $p$  orbitals and the direct exchange between  $p$  and  $d$  orbitals yield a ferromagnetic contribution. However, the former appears at fourth order in the hopping so it was neglected. Only the dominant direct exchange parameter with the  $p_{\parallel}$  orbital,  $K_{\parallel d}$ , was retained. Another simplification was to take a single parameter  $U_p$  for the repulsion of two holes on the same  $p$  orbital or on different  $p$  orbitals. Also for simplicity, we neglected the nearest neighbor repulsion  $U_{pd}$  which can be partially absorbed in the definition of  $\Delta$ .

Because the  $p_z$  orbital is even respect to an exchange of L and R while the  $p_{\parallel}$  is odd, tunneling process though these orbitals interfere destructively as it is clear from the prefactor in Eq. (S8). Clearly, such effect tends to reduce the superexchange interaction  $J^{(4)}$ , respect to a flat configuration ( $t_{zd} = 0$ ).

As a reference, and according to the previous estimates we can take,  $t_{\parallel d} = 1.24$  eV,  $t_{zd} = 0.65$  eV,  $U_d = 9.4$  eV,  $U_p = 4$  eV,  $\Delta = 2.7$  eV. With these parameters and neglecting direct exchange one obtains  $J = J^{(4)} = 0.22$  eV. Such value is too large to be taken seriously but shows that even in the presence of buckling large values of the magnetic interaction are possible. Such overestimation is also common to cuprates when the direct exchange is neglected (49, 61–63). Experimentally  $J = 0.07$  eV is obtained in the main text. This requires  $K_{\parallel d} = -0.17$  eV, which is of the order of typical values in cuprates (49, 61–63).

The above discussion clarifies the role of buckling on the determination of the magnetic interaction. In addition the similarity of microscopic parameters of  $\text{AgF}_2$  with the ones of cuprates have been emphasized and we showed that a large value of  $J$  is not incompatible with the present knowledge of parameters. In the following we present a computation of magnetic interactions based on DFT which confirms this conclusion.

### Density Functional Theory computations and Néel Temperature.

To compute magnetic interactions with DFT one can use either a total energy method (64) (TE) or the magnetic total force theorem (MTFT) (65). The latter has the advantage that interactions of arbitrary range can be computed within one computation. We use the latter as implemented in Ref. 66 for a general exploration of interactions and perform total energy computations to check the results in specific cases.

For the magnetic total force theorem computations, the Green's functions and the local spin-dependent Hamiltonian matrix elements were evaluated using a set of maximally localized Wannier functions calculated with the Wannier90 software interfaced with VASP. This set is different from the Wannier computation of the previous section because only one Wannier orbital per Ag site is retained.

Supplementary Table S2 shows the exchange interactions computed by the two methods. The theoretical nearest neighbor interaction results to be around 1/2 of typical values in cuprates. Despite the fact that some bands in the paramagnetic electronic structure have non-negligibly dispersion in some of the out of plane directions (Supplementary Fig. S3) the magnetic interactions are quite anisotropic.

In order to estimate the Néel temperature we have performed classical Monte Carlo simulations of model Eq. (S6) with spins substituted by classical vectors of length 1/2 and parameters from the MTFT computations. Such simulation yields  $T_N^{\text{class}} = 90$  K. However, treating the spin as classical is a very rough approximation for a spin-1/2 system. To investigate this effect we performed classical simulations of a simple three-dimensional Heisenberg model on a square lattice for which fully quantum mechanical simulations are available (67). Comparing the classical and the quantum simulations for systems of similar ratio of the interlayer to intralayer coupling  $\alpha$  we arrive at the conclusion that the quantum  $T_N = \gamma(\alpha)T_N^{\text{class}}$  with  $\gamma = 2.3$  for the anisotropy of  $\text{AgF}_2$  ( $\gamma$  depends weakly on  $\alpha$  so a precise determination is not necessary). This yields  $T_N = 207$  K for the theoretical Néel temperature of  $\text{AgF}_2$  to be compared with the experimental value  $T_N = 163$  K. Since, as explained in the main text, we find experimentally

that the nearest neighbor magnetic coupling is even larger than the one of the MTFT method we attribute the difference to longer-range coupling. Indeed, we find that such couplings are very sensitive to details of the method while the nearest neighbor coupling is much more robust. For example, using non-optimized Wannier orbitals we find that long-range coupling can change by a factor of 2 while the nearest neighbor coupling changes by 10%. Another source of error may be additional terms in the Hamiltonian not considered here like four-site cyclic exchange (68) and Dzyaloshinsky-Moriya interaction. Given these approximation we find that the theoretical Néel temperature of the same order as the experimental one confirms the presence of robust magnetic interactions in  $\text{AgF}_2$  as in cuprates.

It is natural to ask what would be the exchange constants in hypothetical polymorphs of  $\text{AgF}_2$  that do not have puckering. Possible structures were studied in the past with DFT (46, 69–72). Constraining the  $\text{AgF}_2$  plane to be a mirror plane (but allowing the Ag-F-Ag bond to have an angle inside the plane, Supplementary Table S3) yields the  $\delta\text{-AgF}_2$  polymorph of Refs. 70, 71 with a modest increase in energy at ambient pressure. A large value of  $J$  was predicted for  $\delta\text{-AgF}_2$  with the GGA functional (71) however this may overestimate the magnetic interaction. We have repeated the computation with hybrid-DFT which yields the value in Supplementary Table S3. If one further restricts the bond angles to be straight a tetragonal polymorph is obtained (72) dubbed  $\omega\text{-AgF}_2$ . In this case an even larger nearest neighbor exchange is obtained (Supplementary Table S3). Obviously such polymorphs are not stable at ambient pressure. However, it is possible that they can be stabilized by intercalation or they may be grown as one or few layers on an appropriate substrate.

## Sample preparation

In typical synthesis, 3 g of silver(I) nitrate ( $\text{AgNO}_3$ ) was weighted into the FEP (tetrafluoroethylene-hexafluoropropylene block copolymer) reaction vessel (16 mm i.d., 19 mm. o.d., length = 18 cm; equipped with PTFE valve) in a dry-box. Anhydrous HF (20 ml, Linde, 99.995%), treated with  $\text{K}_2\text{NiF}_6$  (Advance Research Chemicals, Inc.) for several hours prior to use, was condensed onto  $\text{AgNO}_3$  at 77 K. The reaction vessel was brought to ambient temperature and a clear colourless solution was obtained. Elemental fluorine was slowly added at ambient temperature till the pressure in reaction vessel reached 4 bar. Precipitation of brown solid was observed. The stirring of the reaction mixture at ambient temperature was carried out. After one day, the reaction vessel was cooled down to 77 K, volatiles pumped away, reaction mixture brought to ambient temperature and the new portion of fluorine was added. The whole procedure has been repeated several times. With the last portion of fluorine, which was already in an excess the reaction mixture was left for 2–3 days. After that the liquid phase was decanted away and the volatiles were pumped away on overnight at ambient temperature. The freshly prepared sample was used for research as described below. A commercial reference sample of  $\text{AgF}_2$  was obtained from Sigma Aldrich.

## Sample characterization by powder X-ray diffraction

Powder X-ray diffraction pattern (XRD) with  $CoK\alpha$  radiation was recorded at room temperature for freshly prepared and purchased  $AgF_2$  samples enclosed in a 0.3 mm quartz capillary. The XRDs are shown in Supplementary Fig. S5 and indicate the presence of a small amount of  $AgF$  impurity in both samples (reflections from  $AgF$  are somewhat larger in commercial  $AgF_2$  than in a freshly prepared sample) as well as three reflections from unknown impurities (seen only for commercial  $AgF_2$ ; they do *not* originate from  $AgNO_3$ , which is a common precursor of  $AgF_2$ ).

## Sample characterization by heat capacity measurements

Heat capacity measurements were conducted for milligram quantities of  $AgF_2$ . In order to prevent reaction with moisture each sample was wrapped in aluminum foil in a glovebox and then transferred to the Physical Property Measurement System (MPMS, Quantum Design) for measurements. The obtained heat capacities were corrected for the signal from aluminum (72).

The heat capacity of  $AgF_2$  (Supplementary Fig. S6) show a  $\lambda$  type anomaly due to magnetic ordering at 161 K. The entropy change at the phase transition (estimated by integrating  $c_p/T$  at  $\lambda$  peak in the 145–165 K range) equals  $0.28 \text{ J mol}^{-1} \text{ K}^{-1}$ , i.e. only 5 % of  $R\ln(2)$  value expected for full ordering of spin 1/2 system. Thus, the high-T paramagnetic phase must exhibit substantial short-range antiferromagnetic interactions (as for (73)  $CuCl_2$ ). Partial ordering above the Néel point suggest in turn the presence of appreciable magnetic superexchange between the  $Ag^{2+}$  centers.

## Sample characterization by High-Field Electron Paramagnetic Resonance

High-field, high-frequency electron paramagnetic resonance (EPR) spectra at temperatures ranging from ca. 3 K to 290 K were recorded on a home-built spectrometer at the EMR facility of the NHMFL (74). The instrument is equipped with a superconducting magnet (Oxford Instruments) capable of reaching a field of 17 T. Microwave frequencies over the range 52-416 GHz were generated by a phase-locked Virginia Diodes source, producing a base frequency of  $13 \pm 1 \text{ GHz}$ , which was multiplied by a cascade of frequency multipliers. The instrument is a transmission-type device and uses no resonance cavity. A liquid He-cooled InSb bolometer (QMC Instruments Ltd) was used as a microwave detector. All spectra were taken in derivative mode,  $dI/dB$  (where  $I$  is the absorption intensity), using field modulation and a phase-sensitive lock-in detection scheme. Since the samples are moisture-sensitive, they were packed in airtight sample holders ( $\varnothing_{in}=7 \text{ mm}$ ,  $\varnothing_{out}=9 \text{ mm}$ ,  $l=26 \text{ mm}$ ) made from perfluoropolymers, and protected with two tightly fitting PTFE (Teflon<sup>®</sup>) stoppers ( $l=28 \text{ mm}$ ).

We searched for EPR signal using fields from 0 to 14.9 T and frequencies ca. 50-640 GHz at temperatures ranging from ca. 3 K to 200 K and found no signal which could be attributed to the bulk of the sample, a situation that mirrors cuprates (75).

## Raman scattering

Raman spectra shown in Fig. 3 and in Supplementary Fig. S7 were acquired on a dry quartz capillary filled with  $\text{AgF}_2$  in the  $180^\circ$  scattering geometry. The capillary was prefluorinated with  $\text{F}_2$  gas to minimize reactivity towards  $\text{AgF}_2$ . We found that using larger power than the ones reported leads to decomposition of the samples. The following are the instruments used for the data acquisition in the main text: 1) Nicolet 6700/NXR FT-Raman equipped with a Nd:YAG laser for excitation at 1064 nm (1.17 eV), a Nicolet reflective mirror and a liquid nitrogen cooled Ge detector. Spectra were acquired with resolution of  $4\text{ cm}^{-1}$  at 4-5 mW of laser power and referenced to that of elemental silicon. Calibration was done with respect to a standardized built-in Xe lamp. A typical measurement was composed of several thousand accumulations (of ca. 2s each) and took several hours to complete. This configuration has high sensitivity and was used for the weak two-magnon feature at room temperature. 2) Low temperature measurements at identical source/detector combination as in 1) were done in a RFS 100 Bruker Raman interferometer with a resolution of  $4\text{ cm}^{-1}$ . This instrument was calibrated with a black body source at 1273 K placed in the sample position. The incident laser power density was set at  $1.1\text{ W/cm}^2$  (80 mW, ca. 3 mm laser beam diameter). The sample was mounted on the cold finger of a liquid He flow cryostat. Each spectrum is the average of 4000 or 16000 scans (2 or 8 hours). 3) T64000 spectrometer from Horiba-Jobin Yvon equipped with a liquid nitrogen cooled Si detector, and used in the confocal microscope mode (aperture diameter:  $150\text{ }\mu\text{m}$ ) with the Mitutoyo long-working distance lens (focal length of 200 mm). Typical gratings used were 150 lines per mm (preliminary monochromatization stage) and 300 lines per mm (second monochromatization stage). Calibration was done with a black body source at 1200 C placed in the sample position. The 514.5 nm (2.41 eV, 420 mW at head) of a Kr/Ar gas ion laser from Spectra-Physics was used as a source. Spectra were acquired with resolution of  $4.5\text{ cm}^{-1}$  or better, at max. 5 mW of laser power on the cell and referenced to that of diamond or silicon. Filters were used to bring down the beam power at the sample, in some cases down to 0.4 mW. A typical measurement was composed of 340 accumulations (60 s each). 4) Renishaw inVia Raman system with a 785 nm (1.58 eV) line used as the excitation source. The light from the laser was passed through a line filter and focused on the sample mounted on an X-Y-Z translation stage with a  $50\times$  microscope objective. The Raman-scattered light was collected by the same objective through a holographic notch filter to block out Rayleigh scattering. The microscope was equipped with a 1800 grooves per mm grating, cut-off optical filters, and a  $1024\times 256$  pixel Peltier-cooled RenCam CCD detector, which allowed registering the Stokes part of Raman spectra with  $5\text{--}6\text{ cm}^{-1}$  spectral resolution and  $2\text{ cm}^{-1}$  wavenumber accuracy. Calibration was done with a standardized He/Ne lamp. The time required for completing a single Raman spectrum was 4 min with a laser power of 0.25 mW.

## Far infrared absorption spectroscopy

The far infrared (FIR) spectrum has been collected in the transmission mode in a Vertex 80v spectrometer (from Bruker) equipped with a global light source. A mylar beam splitter and DTGS detector were used. The measurement set-up included two PTFE optical windows spaced by a 0.1 mm thin separator; the fine AgF<sub>2</sub> powder was dispersed on the internal side of one of the windows .

## Comparison of phonon frequencies with DFT calculations and mode assignment

We compared the experimental Raman and far infrared (FIR) phonons with the theoretical predictions based on the DFT computations. The purpose is twofold. On one hand, good agreement between theory and experiment allows to validate the accuracy of the DFT computations. On the other hand, AgF<sub>2</sub> can easily decompose due to excessive illumination or reaction with containers or even traces of moisture thus vibration spectroscopy allows to check the integrity of the sample . Including the IR phonons in the analysis ensured that the full phonon assignment is robust. In the following we present both the IR and Raman vibrational analysis.

The unit cell has 4 formula units which yields 36  $\Gamma$ -point frequencies. Symmetry analysis yields the following irreducible representations:

$$\text{AgF}_2 : 3A_g + 6A_u + 3B_{1g} + 6B_{1u} + 3B_{2g} + 6B_{2u} + 3B_{3g} + 6B_{3u}$$

The acoustic modes transform like  $B_{3u}$  ,  $B_{2u}$  and  $B_{1u}$ . Of the remaining modes 15 should be IR active (8 of those are observed), 12 should be Raman active (11 of those are observed), and 6 should be silent.

For the classification of the modes here and in Supplementary Table S4 we adopt a coordination system different from the main paper and such that [AgF<sub>2</sub>] sheets are in the *ac* plane, while *b* axis is perpendicular to them.

Hybrid functional DFT is considered to perform better than DFT+U and was used to obtain more accurate vibrations frequencies but the intensity computation was restricted to the DFT+U method for technical reasons. The theoretical wavenumbers coming from DFT+U calculations or hybrid functional DFT are presented in Supplementary Table S4 as-obtained, i.e. without any scaling to fit the data.

The DFT+U calculations tend to reproduce the IR spectrum reasonably well (Supplementary Fig. S7b). The largest intensity is computed for the 441 cm<sup>-1</sup> band ( $B_{3u}$ ), which is indeed the strongest band in the experimental spectrum (also, its wavenumber is identical to the theoretical value). This band is assigned to  $B_{3u}$  Ag-F stretching mode, which corresponds to local deformation of the local [AgF<sub>4</sub>] square towards the (2+2) bent cis-[F<sub>2</sub>...AgF<sub>2</sub>] unit.

Substantial intensities are also computed for the 453 cm<sup>-1</sup> band (it is too close to the main feature to be distinguished from it clearly) as well as for 310 and 312 cm<sup>-1</sup> bands (there is a

feature at  $307\text{ cm}^{-1}$  in the experimental spectrum), for  $185\text{ cm}^{-1}$  band (exp.  $193\text{ cm}^{-1}$ ), for  $134\text{ cm}^{-1}$  band (there is a shoulder at ca.  $139\text{ cm}^{-1}$  in experimental spectrum) and for  $90\text{ cm}^{-1}$  band (the experimentally seen band at  $93\text{ cm}^{-1}$  is stronger than predicted). The bands seen in experiment at  $159$  and  $168\text{ cm}^{-1}$  have their intensities underestimated by theory (for bands at  $156$  and  $163\text{ cm}^{-1}$ , respectively). Despite these discrepancies, the bands appearing in the experimental spectrum may be rather easily assigned.

Since absolute wavenumbers of the IR-active modes were predicted with the accuracy better than  $10\text{ cm}^{-1}$ , one may base the assignment of Raman-active modes on the assumption that their calculated wavenumbers are fairly correct, too, while the intensities may differ from the experimental ones. This assumption is not unreasonable since Raman intensities are inherently difficult to predict.

The Raman spectra in the phonon region for various excitation energies is shown in Supplementary Figure S7a. The spectra taken with the three laser lines are quite similar. The spectrum taken with  $1064\text{ nm}$  ( $1.17\text{ eV}$ ) excitation is predominated by a strong band at  $254\text{ cm}^{-1}$ , which is assigned to the  $B_{2g}$  mode (for assignment of this and other bands see Supplementary Table S4). Several weaker features appear, particularly at  $168$ ,  $183$ ,  $198$ ,  $314$ , and  $486\text{ cm}^{-1}$ . The broad band at ca.  $970\text{ cm}^{-1}$  is also seen.

For the excitation with  $514.5\text{ nm}$  ( $2.41\text{ eV}$ ) a mode at  $417\text{ cm}^{-1}$  relatively gains on intensity. Since the intensity of this mode grows with the photon dose we assign it to an impurity phase generated via a photochemical processes. The absence of this band was monitored to check the integrity of the sample for both vibrational and electronic Raman measurements.

Importantly, the strongest calculated Raman band at  $253\text{ cm}^{-1}$  is found at  $254\text{-}258\text{ cm}^{-1}$  in the experimental spectra. This band is assigned to the  $B_{2g}$  mode involving the Ag-F stretching, which leads to the formation of quasi-1D kinked-chain structure  $(\text{AgF}^+)(\text{F}^-)$ . The relative intensities of four Raman-active bands in its vicinity are not predicted very accurately, as expected, but their wavenumbers agree very well with the experimental values ( $311\text{ exp. vs. }309\text{ cm}^{-1}\text{ theor.}$ ;  $290\text{ exp. vs. }296\text{ cm}^{-1}\text{ theor.}$ ;  $244\text{ exp. vs. }249\text{ cm}^{-1}\text{ theor.}$ ;  $232\text{ exp. vs. }227\text{ cm}^{-1}\text{ theor.}$ ). The last important band which is predicted to be quite intense in Raman spectrum is the one positioned at  $443\text{ cm}^{-1}$  ( $B_{2g}$ ). We find a weak Raman feature at  $446\text{ cm}^{-1}$  in some of our spectra, which we tentatively assign to this  $B_{2g}$  mode.

Having assigned fundamentals, it is now possible to understand the origin of the broad structured band appearing at  $970\text{ cm}^{-1}$  in spectra measured with  $1064\text{ nm}$  or  $514.5\text{ nm}$  excitation (see main paper). This band likely originates from the first overtones of the highest-frequency Raman ( $B_{3g}$   $478\text{ cm}^{-1}$ ,  $B_{2g}$   $481\text{ cm}^{-1}$ ), IR-active ( $B_{1u}$   $470\text{ cm}^{-1}$ ,  $B_{2u}$   $468\text{ cm}^{-1}$ ) and silent modes ( $A_u$   $477\text{ cm}^{-1}$ ). The first overtones for all of them are totally symmetric ( $A_g$ ) and likely resonance-enhanced, particularly at  $514.5\text{ nm}$  excitation. Since two phonons are combined the total momentum of the pair is restricted to be zero but one of the constituents can have arbitrary momentum which explains the broad structure.

Respect to the group theory analysis, 1 extra band appears in the IR spectrum (shoulder at  $497\text{ cm}^{-1}$ ), and 4 extra bands in Raman spectra ( $138\text{ cm}^{-1}$ ,  $368\text{-}377$ ,  $413\text{-}419$ , and  $480\text{-}485\text{ cm}^{-1}$ ). In Supplementary Table S4 we propose their assignment to the corresponding overtones

and/or combination modes, using match of wavenumbers and symmetry considerations.

Based on the analyses presented above, supplemented by more thorough analysis of all weak features, we obtain the band assignment shown in Supplementary Table S4.

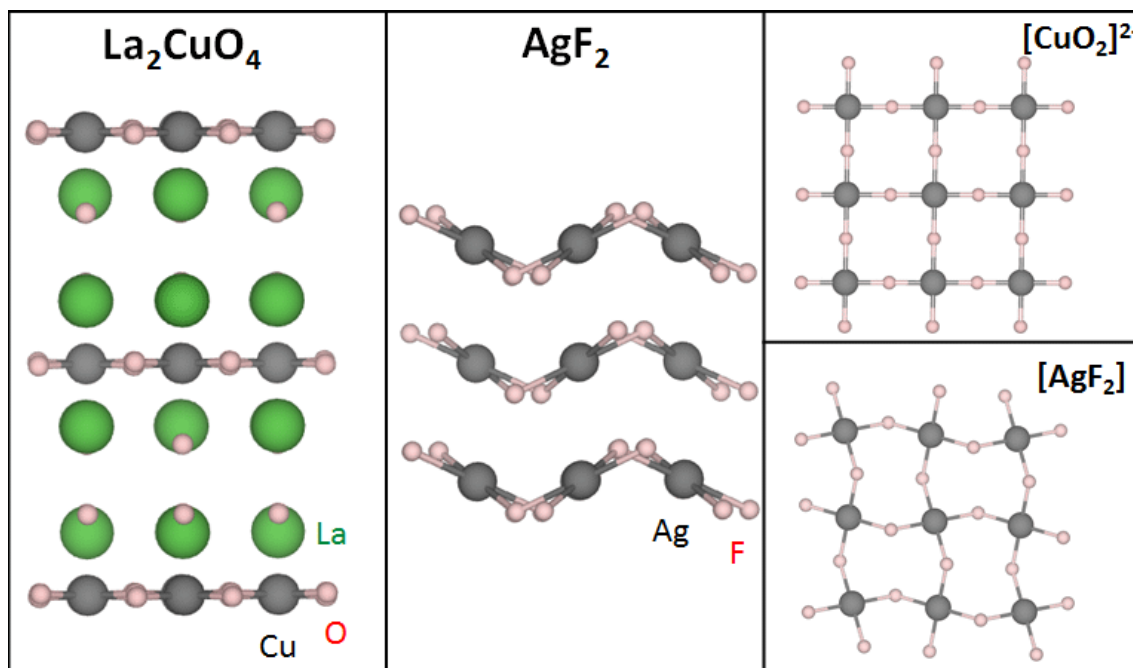

Figure S1: **Comparison of the crystal structure of  $\text{La}_2\text{CuO}_4$  and  $\text{AgF}_2$ .** Notice that for the cuprate layers formed of charged  $[\text{CuO}_4]^{-6}$  units are compensated by the  $[\text{La}_2]^{+6}$  spacer layers. Instead, the  $[\text{AgF}_2]$  layers are intrinsically neutral and charged spacing layers are not required. Notice the similarity of the sheet topology shown on the right panels.

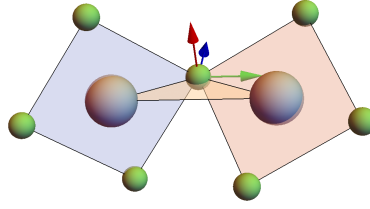

Figure S2: **Schematic representation of an Ag-F-Ag bond** Gray (green) spheres represent Ag (F) atoms.  $d_{x^2-y^2}$  orbitals are label as  $d_L$  and  $d_R$  for the left and right Ag respectively. They are defined in such a way that the lobes are oriented approximately along the diagonals of the approximate squares defined by F's (light blue and salmon). We also show the triangle defined by the central F and the two Ag's. The arrows represent the direction taken for the  $p$  orbitals ( $p_{\perp}, p_{\parallel}, p_z$ ). Red is orthogonal to the triangle plane and defines the  $p_{\perp}$  orbital. Green ( $p_{\parallel}$ ) is parallel to the Ag-Ag bond while blue ( $p_z$ ) is contained in the triangle plane, is perpendicular to the Ag-Ag bond and points approximately in the  $c$  direction.

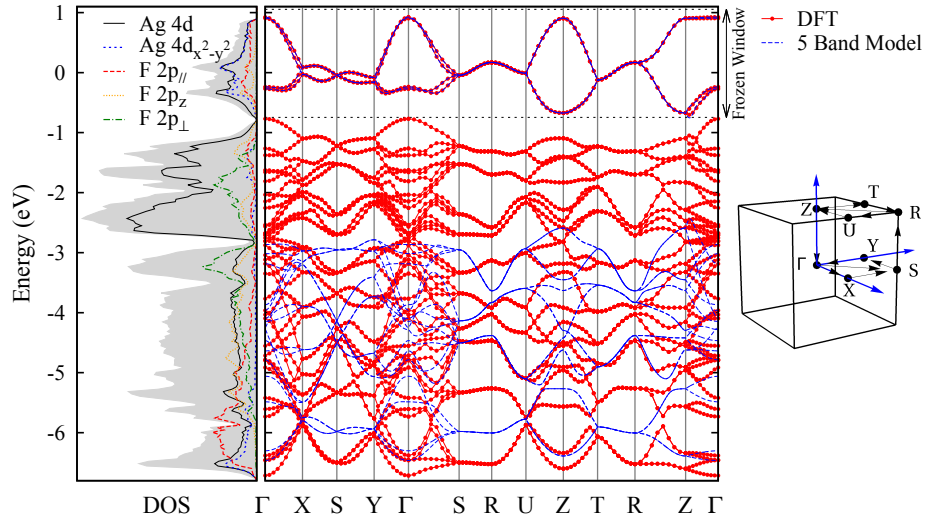

Figure S3: **Unpolarized band structure of  $\text{AgF}_2$ .** The right panel show the DFT bands obtained with VASP in the region dominated by F-2p and Ag-4d orbitals (red) and the bands obtained with the Wannier90 code (blue) using a Wannier basis with one  $d$  and four  $p$  orbitals per formula unit (5-band model). Wannier orbitals are optimized to match the bands within the indicated frozen window. This provides accurate bands around the the Fermi energy which is located at zero energy. The inset shows schematically the path around the Brillouin zone. The filled gray curve in the left panel is the total density of states (DOS) while the other curves are the orbital resolved DOS.

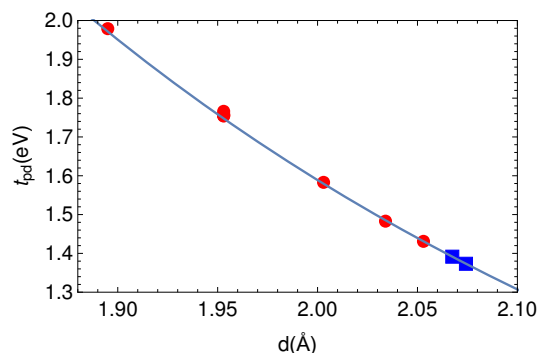

Figure S4: **Hopping matrix elements vs. F-Ag distance ( $d$ )** Red dots are from Refs. 45, 46. Extrapolation was done assuming Andersen scaling (47),  $(pd\sigma) = (pd\sigma)^0(d_0/d)^4$  (blue line). The blue dots are the  $t_{pd}$  values estimated for the two possible Ag-F distances in  $\text{AgF}_2$ .

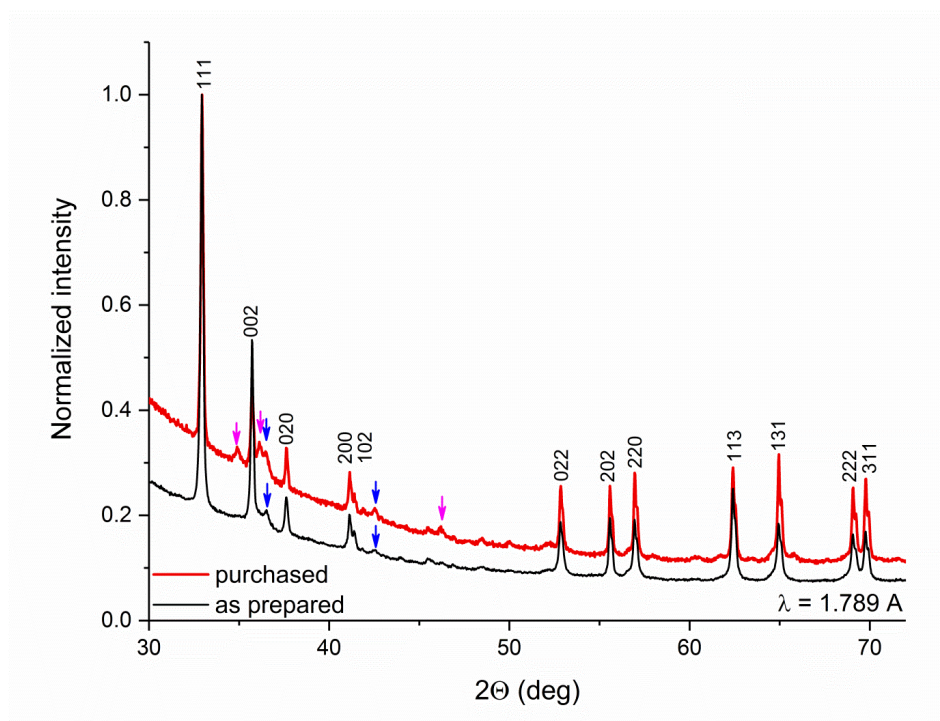

Figure S5: **X-ray characterization.** Comparison of X-ray diffraction patterns ( $\lambda(\text{K}\alpha_1) = 1.7890 \text{ \AA}$ , Co) for as-synthesized (black line) and commercial (red line)  $\text{AgF}_2$ . Blue arrows mark reflections coming from  $\text{AgF}$ , pink – from unknown impurities. The hkl indices from  $\text{AgF}_2$  are given. No reflections are seen for  $2\theta < 30^\circ$  hence this region is not shown here.

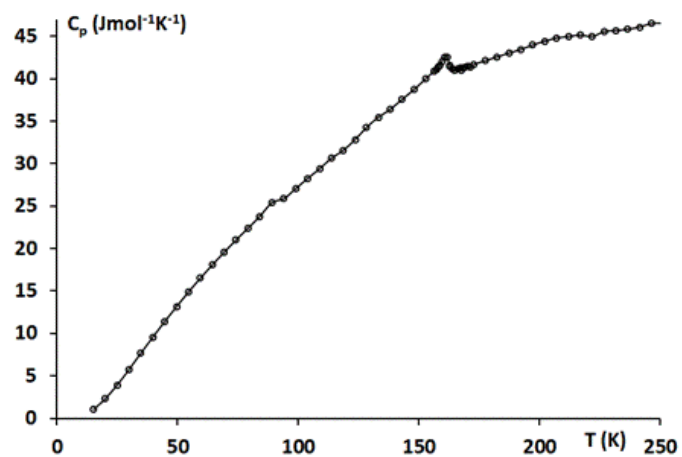

Figure S6: **Heat capacity of  $\text{AgF}_2$  as a function of temperature.** The  $\lambda$  peak with the maximum at 161 K has been used for the estimate of magnetic entropy change at the phase transition.

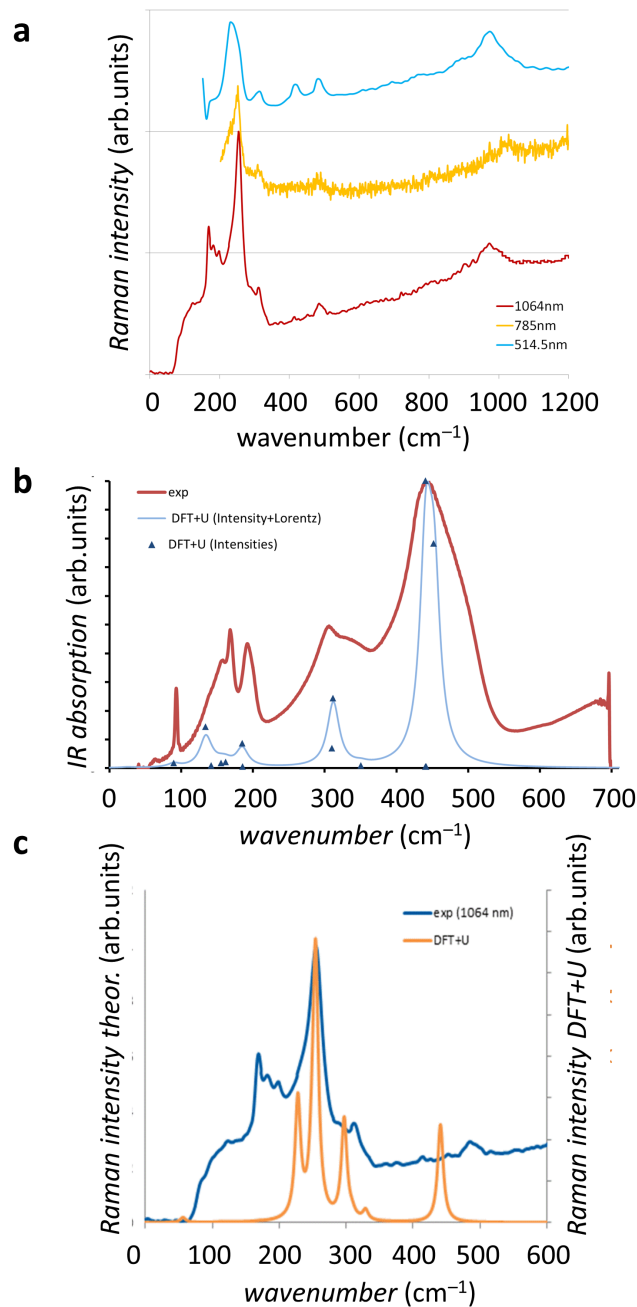

Figure S7: **Vibrational spectroscopy.** **a** The Raman spectra of AgF<sub>2</sub> measured at different excitation lines. We show the range of fundamental modes (up to ca. 490 cm<sup>-1</sup>) and overtones (up to ca. 970 cm<sup>-1</sup>). **b** Comparison of the measured (red line) and simulated using Lorentzian functions (blue line) IR absorption spectrum of AgF<sub>2</sub> (green triangles mark the positions of IR-active modes calculated at DFT+U level, dark blue triangles mark their calculated intensities, which were used for generating of the simulated spectrum). **c** Comparison of the measured (blue line) and simulated (orange line) Raman spectrum of AgF<sub>2</sub>.

|               | $t_{  dl}$ | $t_{  ds}$ | $t_{zdl}$ | $t_{zds}$ |
|---------------|------------|------------|-----------|-----------|
| Slater-Koster | 1.24       | 1.26       | 0.58      | 0.59      |
| 1+4 orbitals  | 1.20       | 1.28       | 0.73      | 0.58      |
| 5+6 orbitals  | 1.25       | 1.26       | 0.56      | 0.60      |

Table S1: **Nearest neighbor pd hopping integrals (eV).** Slater-Koster are the results extrapolated from the DFT computations of Ref. 45, 46 and Eq. (S4). The next two lines show the present Wannier90 computations with 5 and 11 orbitals per f.u. The subindex  $s/l$  refers to the non-equivalent short and long bonds present in the structure.

| Mult. | Position diff. |           |           | $J_{ij}$ (MTFT) | $J_{ij}$ (TE) |
|-------|----------------|-----------|-----------|-----------------|---------------|
|       | <b>a</b>       | <b>b</b>  | <b>c</b>  | meV             | meV           |
| 4     | $\pm 0.5$      | $\pm 0.5$ | 0         | 52              | 56            |
| 2     | 0              | $\pm 1$   | 0         | 4.5             | -             |
| 2     | $\pm 1$        | 0         | 0         | 4.2             | -             |
| 2     | $\pm(1$        | $-1)$     | 0         | 1.2             | -             |
| 2     | $\pm(1$        | $1)$      | 0         | 1.1             | -             |
| 4     | $\pm(0.5$      | $-1)$     | $\pm 0.5$ | 0.45            | -             |
| 2     | 0              | $\pm(1$   | $-1)$     | -0.26           | -             |
| 4     | $\pm(0.5$      | $1)$      | $\pm 0.5$ | 0.11            | -             |
| 4     | 0              | $\pm 0.5$ | $\pm 0.5$ | 0.576           | -1.62         |
| 4     | $\pm 0.5$      | 0         | $\pm 0.5$ | -0.15           | -1.01         |
| 4     | $\pm(1$        | $0.5)$    | $\pm 0.5$ | -0.16           | -             |

Table S2: **Magnetic exchange constant** We show the exchange constant  $J_{ij}$  computed with the MTFT method (66) and with the TE method (64) for specific directions. Columns 2-4 are the difference in the position of Ag ions  $i$  and  $j$  in lattice units. In plane exchange constants less than 1 meV were neglected. The first column are the number of bonds with the same exchange matrix element (fixing the initial atom).  $\pm(1 -1)$  is a shorthand for  $1 -1$  and  $-1 1$ .

|                            | Cell vectors (Å) |                  |                  | $R_{Ag-F-Ag}$ | $\eta$ | $J$        |
|----------------------------|------------------|------------------|------------------|---------------|--------|------------|
|                            | $a$              | $b$              | $c$              | (Å)           |        | (meV)      |
| $\alpha$ -AgF <sub>2</sub> | 5.191<br>(5.101) | 5.662<br>(5.101) | 6.042<br>(5.831) | 4.198         | 132.4° | 56<br>(70) |
| $\delta$ -AgF <sub>2</sub> | 5.671            | 5.670            | 5.607            | 4.166         | 148.5° | 137        |
| $\omega$ -AgF <sub>2</sub> | 5.836            | 5.836            | 6.213            | 4.127         | 180°   | 195        |

Table S3: **Exchange constants for AgF<sub>2</sub> and its two hypothetical polymorphs.** We report key structural parameters and values of the nearest neighbour magnetic coupling constant calculated with the total energy method.  $R_{Ag-F-Ag}$  is the sum of the two Ag-F distances of the bond.  $\alpha$ -AgF<sub>2</sub> is the known stable phase in which experiments have been done (experimental values are given in parenthesis).  $\omega$ -AgF<sub>2</sub> is tetragonal but cell parameters are reported in the  $\sqrt{2} \times \sqrt{2} \times 1$  unit cell for comparison. See text for a detailed description of the polymorphs.

| No. | Exp.IR | Exp. Raman | DFT+U | HSE06 | Symm. (activity) | Comment                                                                 |
|-----|--------|------------|-------|-------|------------------|-------------------------------------------------------------------------|
| 1   | 497sh  |            |       |       |                  | 441+56 combination ( $B_{3u}$ )<br>and/or 470 IR $B_{2u}$ (HSE06)       |
| 2   |        | 480-485    |       |       |                  | 254+233 combination ( $B_{2g}$ )<br>and/or 481 Raman $B_{2g}$ (HSE06)   |
| 3   |        |            | 461   | 477   | $A_u$ (silent)   |                                                                         |
| 4   |        |            | 455   | 470   | $B_{2u}$ (IR)    |                                                                         |
| 5   |        |            | 453   | 468   | $B_{1u}$ (IR)    |                                                                         |
| 6   |        | 446        | 443   | 481   | $B_{2g}$ (Raman) |                                                                         |
| 7   | 441vs  |            | 441   | 459   | $B_{3u}$ (IR)    |                                                                         |
| 8   |        |            | 441   | 478   | $B_{3g}$ (Raman) |                                                                         |
| 9   |        | 413-419    |       |       |                  | 341+73 combination ( $B_{3g}$ )<br>& photochemical product*             |
| 10  |        | 368-377    |       |       |                  | 193+168 combination ( $B_{1g}$ )<br>and/or 193 first overtone ( $A_g$ ) |
| 11  | 341sh  |            | 350   | 356   | $B_{3u}$ (IR)    |                                                                         |
| 12  |        | 337        | 329   | 340   | $B_{1g}$ (Raman) |                                                                         |
| 13  |        |            | 323   | 325   | $A_u$ (silent)   |                                                                         |
| 14  | 307m   |            | 312   | 317   | $B_{2u}$ (IR)    |                                                                         |
| 15  | 307m   |            | 310   | 317   | $B_{1u}$ (IR)    |                                                                         |
| 16  |        | 311-312    | 309   | 323   | $A_g$ (Raman)    |                                                                         |
| 17  |        | 290-291    | 296   | 307   | $B_{1g}$ (Raman) |                                                                         |
| 18  |        | 258        | 253   | 257   | $B_{2g}$ (Raman) |                                                                         |
| 19  |        | 244        | 249   | 250   | $B_{3g}$ (Raman) |                                                                         |
| 20  |        | 232-233    | 227   | 232   | $A_g$ (Raman)    |                                                                         |
| 21  | 193m   |            | 186   | 199   | $B_{2u}$ (IR)    |                                                                         |
| 22  | 193m   |            | 185   | 195   | $B_{1u}$ (IR)    |                                                                         |
| 23  |        |            | 183   | 200   | $A_u$ (silent)   |                                                                         |
| 24  |        | 162-174    | 171   | 183   | $B_{2g}$ (Raman) |                                                                         |
| 25  | 168m   |            | 163   | 175   | $B_{3u}$ (IR)    |                                                                         |
| 26  |        |            | 162   | 170   | $A_u$ (silent)   |                                                                         |
| 27  | 159w   |            | 156   | 161   | $B_{3u}$ (IR)    |                                                                         |
| 28  |        |            | 143   | 146   | $B_{1u}$ (IR)    |                                                                         |
| 29  | 139sh  |            | 134   | 136   | $B_{2u}$ (IR)    |                                                                         |
| 30  |        | 138        |       |       |                  | 73+73 first overtone ( $A_g$ )                                          |
| 31  |        | 125        | 132   | 140   | $B_{3g}$ (Raman) |                                                                         |
| 32  |        | 102-117    | 115   | 118   | $B_{1g}$ (Raman) |                                                                         |
| 33  |        |            | 98    | 101   | $A_u$ (silent)   |                                                                         |
| 34  | 93w    |            | 94    | 93    | $B_{3u}$ (IR)    |                                                                         |
| 35  | 93w    |            | 90    | 92    | $B_{1u}$ (IR)    |                                                                         |
| 36  |        |            | 73    | 72    | $A_u$ (silent)   |                                                                         |
| 37  |        | 57         | 59    | 65    | $A_g$ (Raman)    |                                                                         |
| 38  | —      |            | 27    | 38    | $B_{2u}$ (IR)    | range not measured                                                      |

**Table S4: Experimental and Theoretical Phonon Frequencies** We provide a tentative assignment of bands appearing in the IR and Raman spectra of  $AgF_2$  (wavenumbers in  $cm^{-1}$ ). We classify the modes as shoulder (sh), very strong (vs), strong(s), medium (m) and weak (w). \*Intensity of this band clearly grows with the illumination time; the nature of chemical species which is the product of photochemical decomposition will be elucidated elsewhere.

## References

31. K. Momma, F. Izumi, VESTA 3 for three-dimensional visualization of crystal, volumetric and morphology data, *J. Appl. Crystallogr.* **44**, 1272 (2011).
32. P. Charpin, P. Plurien, P. Meriel, A neutron diffraction study of crystal and magnetic structure of  $\text{AgF}_2$ , *Bull. Soc. Fr. Miner. Cristal.* **93**, 7 (1970).
33. P. Fischer, D. Schwarzenbach, H. Rietveld, Crystal and magnetic structure of silver difluoride, *J. Phys. Chem. Solids* **32**, 543 (1971).
34. A. Jesih, K. Lutar, B. Zemva, B. Bachmann, S. Becker, B. G. Müller, R. Hoppe, Einkristalluntersuchungen an  $\text{AgF}_2$ , *Z. Anorg. Allg. Chem.* **588**, 77 (1990).
35. G. Kresse, J. Furthmüller, Efficient iterative schemes for ab initio total-energy calculations using a plane-wave basis set, *Phys. Rev. B* **54**, 11169 (1996).
36. J. P. Perdew, K. Burke, M. Ernzerhof, Generalized gradient approximation made simple, *Phys. Rev. Lett.* **77**, 3865 (1996).
37. P. Fischer, G. Roullet, D. Schwarzenbach, Crystal and magnetic structure of silver difluoride-II. Weak 4d-ferromagnetism of  $\text{AgF}_2$ , *J. Phys. Chem. Solids* **32**, 1641 (1971).
38. A. V. Krukau, O. A. Vydrov, A. F. Izmaylov, G. E. Scuseria, Influence of the exchange screening parameter on the performance of screened hybrid functionals, *J. Chem. Phys.* **125**, 224106 (2006).
39. P. Giannozzi, S. Baroni, Vibrational and dielectric properties of  $\text{C}_{60}$  from density-functional perturbation theory, *J. Chem. Phys.* **100**, 8537 (1994).
40. K. Esfarjani, Y. Hashi, J. Onoe, K. Takeuchi, Y. Kawazoe, Vibrational modes and IR analysis of neutral photopolymerized  $\text{C}_{60}$  dimers, *Phys. Rev. B* **57**, 223 (1998).
41. D. Karhánek, T. Bučko, J. Hafner, A density functional study of the adsorption of methanethiol on the (111) surfaces of the Ni-group metals: I. Molecular and dissociative adsorption, *J. Phys. Condens. Matter* **22** (2010).
42. A. Fonari, S. Stauffer, *vasp\_raman\_py* (<https://github.com/raman-sc/VASP/>, 2013).
43. V. J. Emery, Theory of high- $T_c$  superconductivity in oxides, *Phys. Rev. Lett.* **58**, 2794 (1987).
44. J. C. Slater, G. F. Koster, Simplified LCAO method for the periodic potential problem, *Phys. Rev.* **94**, 1498 (1954).

45. X. Yang, H. Su, Cuprate-like electronic properties in superlattices with  $\text{Ag(II)F}_2$  square sheet., *Sci. Rep.* **4**, 5420 (2014).
46. X. Yang, H. Su, Electronic Properties of Fluoride and Half-fluoride Superlattices  $\text{KZnF}_3/\text{KAgF}_3$  and  $\text{SrTiO}_3/\text{KAgF}_3$ , *Sci. Rep.* **5**, 15849 (2015).
47. O. K. Andersen, W. Klose, H. Nohl, Electronic structure of Chevrel-phase high-critical-field superconductors, *Phys. Rev. B* **17**, 1209 (1978).
48. N. Marzari, A. a. Mostofi, J. R. Yates, I. Souza, D. Vanderbilt, Maximally localized Wannier functions: Theory and applications, *Rev. Mod. Phys.* **84**, 1419 (2012).
49. A. K. McMahan, J. F. Annett, R. M. Martin, Cuprate parameters from numerical Wannier functions, *Phys. Rev. B* **42**, 6268 (1990).
50. D. K. G. De Boer, C. Haas, G. A. Sawatzky, Exciton satellites in photoelectron spectra, *Phys. Rev. B* **29**, 4401 (1984).
51. J. Ghijsen, L. Tjeng, J. van Elp, H. Eskes, J. Westerink, G. Sawatzky, M. Czyzyk, Electronic structure of  $\text{Cu}_2\text{O}$  and  $\text{CuO}$ , *Phys. Rev. B* **38**, 11322 (1988).
52. L. H. Tjeng, M. B. J. B. Meinders, J. van Elp, J. Ghijsen, G. A. Sawatzky, R. L. Johnson, Electronic structure of  $\text{Ag}_2\text{O}$ , *Phys. Rev. B* **41**, 3190 (1990).
53. J. van den Brink, M. Meinders, J. Lorenzana, R. Eder, G. A. Sawatzky, New Phases in an Extended Hubbard Model Explicitly Including Atomic Polarizabilities, *Phys. Rev. Lett.* **75**, 4658 (1995).
54. J. R. Tessman, A. H. Kahn, W. Shockley, Electronic Polarizabilities of Ions in Crystals, *Phys. Rev.* **92**, 890 (1953).
55. M. Cini, Density of states of two interacting holes in a solid, *Solid State Commun.* **20**, 605 (1976).
56. G. A. Sawatzky, Quasiatomic auger spectra in narrow-band metals, *Phys. Rev. Lett.* **39**, 504 (1977).
57. E. Antonides, E. C. Janse, G. A. Sawatzky, LMM Auger spectra of Cu, Zn, Ga, and Ge. I. Transition probabilities, term splittings, and effective Coulomb interaction, *Phys. Rev. B* **15**, 1669 (1977).
58. C. J. Powell, Solid-state features in the valence band Auger spectra of copper, silver and gold, *Solid State Commun.* **26**, 557 (1978).
59. A. C. Parry-Jones, P. Weightman, P. T. Andrews, The  $\text{M}_{4,5}\text{N}_{4,5}\text{N}_{4,5}$  Auger spectra of Ag, Cd, In and Sn, *J. Phys. C Solid State Phys.* **12**, 1587 (1979).

60. P. Anderson, Antiferromagnetism. Theory of superexchange interaction, *Phys. Rev.* **79**, 350 (1950).
61. M. Braden, G. Wilkendorf, J. Lorenzana, M. Aïn, G. J. McIntyre, M. Behruzi, G. Heger, G. Dhalenne, A. Revcolevschi, Structural analysis of  $\text{CuGeO}_3$ : Relation between nuclear structure and magnetic interaction, *Phys. Rev. B* **54**, 1105 (1996).
62. E. B. Stechel, D. R. Jennison, Electronic structure of  $\text{CuO}_2$  sheets and spin-driven high- $T_c$  superconductivity, *Phys. Rev. B* **38**, 4632 (1988).
63. H. Eskes, J. H. Jefferson, Superexchange in the cuprates, *Phys. Rev. B* **48**, 9788 (1993).
64. R. L. Martin, F. Illas, Antiferromagnetic Exchange Interactions from Hybrid Density Functional Theory, *Phys. Rev. Lett.* **79**, 1539 (1997).
65. A. I. Liechtenstein, M. I. Katsnelson, V. P. Antropov, V. A. Gubanov, Local spin density functional approach to the theory of exchange interactions in ferromagnetic metals and alloys, *J. Magn. Magn. Mater.* **67**, 65 (1987).
66. D. M. Korotin, V. V. Mazurenko, V. I. Anisimov, S. V. Streltsov, Calculation of the exchange constants of the Heisenberg model in the plane-wave based methods using the Green's function approach, *Phys. Rev. B* **91**, 224405 (2014).
67. P. Sengupta, A. W. Sandvik, R. R. P. Singh, Specific heat of quasi-two-dimensional antiferromagnetic Heisenberg models with varying interplanar couplings, *Phys. Rev. B* **68**, 094423 (2003).
68. J. Lorenzana, J. Eroles, S. Sorella, Does the Heisenberg Model Describe the Multimagnon Spin Dynamics in Antiferromagnetic  $\text{CuO}$  Layers?, *Phys. Rev. Lett.* **83**, 5122 (1999).
69. W. Grochala, On similarities and differences of the electronic structure for  $\text{Cu(II)/O}^{2-}$  and  $\text{Ag(II)/F}^{1-}$  infinite layer compounds, *Scr. Mater.* **55**, 811 (2006).
70. J. Romiszewski, W. Grochala, L. Z. Stolarczyk, Pressure-induced transformations of  $\text{Ag II F 2}$  —towards an 'infinite layer' d 9 material, *J. Phys. Condens. Matter* **19**, 116206 (2007).
71. T. Jaroń, W. Grochala, Prediction of giant antiferromagnetic coupling in exotic fluorides of Ag, *Phys. Status Solidi - Rapid Res. Lett.* **2**, 71 (2008).
72. D. Kurzydłowski, PhD Thesis, Ph.D. thesis, Univ. of Warsaw, Poland (2013).
73. M. G. Banks, R. K. Kremer, C. Hoch, A. Simon, B. Ouladdiaf, J. M. Broto, H. Rakoto, C. Lee, M. H. Whangbo, Magnetic ordering in the frustrated Heisenberg chain system cupric chloride  $\text{CuCl}_2$ , *Phys. Rev. B - Condens. Matter Mater. Phys.* **80** (2009).

74. A. Hassan, L. Pardi, J. Krzystek, A. Sienkiewicz, P. Goy, M. Rohrer, L.-C. Brunel, Ultrawide Band Multifrequency High-Field EMR Technique: A Methodology for Increasing Spectroscopic Information, *J. Magn. Reson.* **142**, 300 (2000).
75. P. Simon, J. M. Bassat, S. B. Oseroff, Z. Fisk, S. W. Cheong, A. Wattiaux, S. Schultz, Absence of  $\text{Cu}^{2+}$  electron-spin resonance in high-temperature superconductors and related insulators up to 1150 K, *Phys. Rev. B* **48**, 4216 (1993).
